# Supplementary material for: Reward Prediction Error as an Exploration Objective in Deep RL
Source: arXiv:1906.08189 source file (2021-01-14)
Supplement: Supplementary file 1 [file supp.tex]

\appendix
\section{Implementation Details and Hyperparameters}
\label{appendix:implementation}

\begin{table}[t]
\caption{Parameters used for benchmark runs.}
\label{hyper-table}
\vskip 0.15in
\begin{center}
\begin{small}
\begin{sc}
\begin{tabular}{lcccr}
\toprule

Default Parameters \\
\midrule
CEM  \\
\hspace{5mm} iterations      & 4 \\
\hspace{5mm} number of samples      & 64 \\
\hspace{5mm} top k & 6 \\
All Networks\\
\hspace{5mm} neurons per layer & 256\\
\hspace{5mm} number of layers & 3\\
\hspace{5mm} non-linearities & ReLU\\
\hspace{5mm} Optimizer & Adam \\
\hspace{5mm} Adam momentum terms & $\beta_1 = 0.9, \beta_2 = 0.99$ \\
Training \\
\hspace{5mm} Q learning rate & 0.001 \\
\hspace{5mm} batch size & 128 \\
\hspace{5mm} time decay $\gamma$ & 0.99 \\
\hspace{5mm} target Q-function update $\tau$ & 0.005 \\
\hspace{5mm} target update frequency & 2 \\
\hspace{5mm} TD3 policy noise & 0.2 \\
\hspace{5mm} TD3 noise clip & 0.5 \\
\hspace{5mm} training steps per env timestep & 1 \\
QXplore-specific \\
\hspace{5mm} $Q_x$ learning rate & 0.001 \\
\hspace{5mm} $Q$ batch data ratio & 0.75 \\
\hspace{5mm} $Q_x$ batch data ratio & 0.75 \\
\hspace{5mm} $\beta_Q$ (Q initial output bias) & 0 \\
RND-specific \\
\hspace{5mm} predictor network learning rate & 0.001 \\
\hspace{5mm} Extrinsic reward weight & 2 \\
\hspace{5mm} Intrinsic reward weight & 1 \\
\hspace{5mm} $\gamma_{\text{E}}$ & 0.99 \\
\hspace{5mm} $\gamma_{\text{I}}$ & 0.99 \\
DORA-specific \\
\hspace{5mm} $\epsilon$ & 0.1 \\
\hspace{5mm} $\beta$ & 0.05 \\
\hspace{5mm} $\gamma_{\text{E}}$ & 0.99 \\
\hspace{5mm} $\gamma_{\text{Q}}$ & 0.99 \\
$\epsilon$-greedy-specific \\
\hspace{5mm} $\epsilon$ & 0.1 \\

\bottomrule
\end{tabular}
\end{sc}
\end{small}
\end{center}
\vskip -0.1in
\end{table}

We describe here the details of our implementation and training parameters. We held these factors constant and used a shared codebase for QXplore, RND, and $\epsilon$-greedy to enable a fair comparison. We used an off-policy Q-learning method based off of TD3 \citep{fujimoto2018td3} and CGP \citep{simmons2019q} with twin Q-functions and a cross-entropy method policy for better hyperparameter robustness. Each network ($Q_{\theta}$, $Q_{x,\phi}$, RND's random and predictor networks) consisted of a 4-layer MLP of 256 neurons per hidden layer, with ReLU non-linearities. We used a batch size of 128 and learning rate of 0.001, and for QXplore sampled training batches for $Q$ and $Q_x$ of 75\% self-collected data and 25\% data collected by the other Q-function's policy as described in Algorithm \ref{alg:qxplore}. 

For DORA \citep{fox2018dora}, we used the hyperparameters and training procedure specified by the original paper where possible, though it was necessary to adapt the method somewhat to the continuous action domain. This is because the original formulation proscribed an ``LLL'' action selection scheme that requires taking discrete log-probabilities of the distribution of Q and E values over actions, which is not tractable in continuous action spaces. Instead, we tried selecting actions using either a CEM policy that maximizes the sum of the two objectives, or using the E values as a reward bonus for training Q and selecting actions that maximize Q only. We thus expect the performance of our implementations to be somewhat worse than a hypothetical distributional-DORA, though the action selection scheme we used does make this version directly comparable to QXplore and RND. Both formulations behaved similarly on \texttt{SparseHalfCheetah} and did not achieve reward with any frequency.

For $\epsilon$-greedy sampling with continuous actions, we sampled a uniform distribution of the valid action range (-1 to 1 for all tasks) with probability $\epsilon$ and act greedily otherwise. We note that the stochastic cross-entropy method policies we used for all experiments also introduce some amount of local exploration through noisy action selection.

We present the parameters we used for the benchmark tasks in Table \ref{hyper-table}.

\section{Environment Details}
\label{appendix:environment_details}
 We use the \texttt{SparseHalfCheetah} environment proposed by \cite{houthooft2016vime} in which a simulated cheetah receives a reward of 0 if it is at least 5 units forward from the initial position and otherwise receives a reward of -1. We also use the OpenAI gym tasks, \texttt{FetchPush}, \texttt{FetchSlide}, and \texttt{FetchPickAndPlace}, which were originally developed for benchmarking HER \citep{andrychowicz2017her}. The objective in these environments is to move a block to a target position, with a reward function returning -1 if the block is not at the target and 0 if it is at the target. For consistency in reward shaping, we structured the reward function of the \texttt{SparseHalfCheetah} task to match the \texttt{Fetch} tasks, such that the baseline reward level is -1 while a successful state provides 0 reward, but report reward values on a 0 to 500 scale for direct comparison with previous work. We trained each method with 5 random seeds for 5,000 episodes on \texttt{SparseHalfCheetah} and 50,000 episodes on \texttt{Fetch} tasks. Time to convergence on these tasks for any exploration method is highly variable, and as such we visualize the mean and standard deviation of the runs in our results.
 
 \section{Ablations}
\label{appendix:ablations}
To study the effects of different components of QXplore, we performed several ablations, as discussed in Section \ref{subsec:ablations}. First, we replaced $Q_{\theta}$ with simple 1-step reward prediction, and $Q_x$'s objective function with maximizing cumulative 1-step reward prediction error plus extrinsic reward, which we label as ``QXplore-1-step'' in Figure \ref{fig:ablations}. This ablation fails to find reward, as the 1-step reward prediction error makes long range exploration more difficult to learn. 

\begin{figure}[ht]
%\vskip 0.2in
\begin{center}

%\vskip 0.2in
    % \begin{subfigure}[b]{0.45\textwidth}
    %     \centering
    %     % \includegraphics[width=\textwidth]{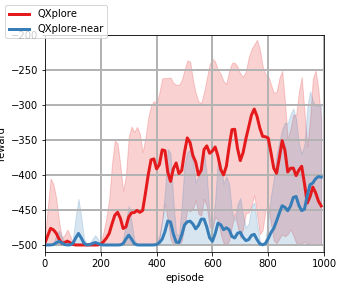}
    %     \includegraphics[width=\textwidth]{figures/benchmarks/ablation.png}

    %     \caption{\label{fig:figd} SparseHalfCheetah}
    % \end{subfigure}
    %     \begin{subfigure}[b]{0.45\textwidth}
    %     \centering
    %     \includegraphics[width=\textwidth]{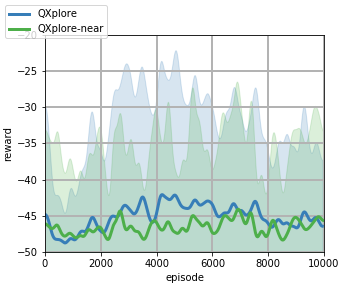}
    %     \caption{\label{fig:figf} FetchPush-v1}
    % \end{subfigure}
    
\centering
\includegraphics[width=0.45\textwidth]{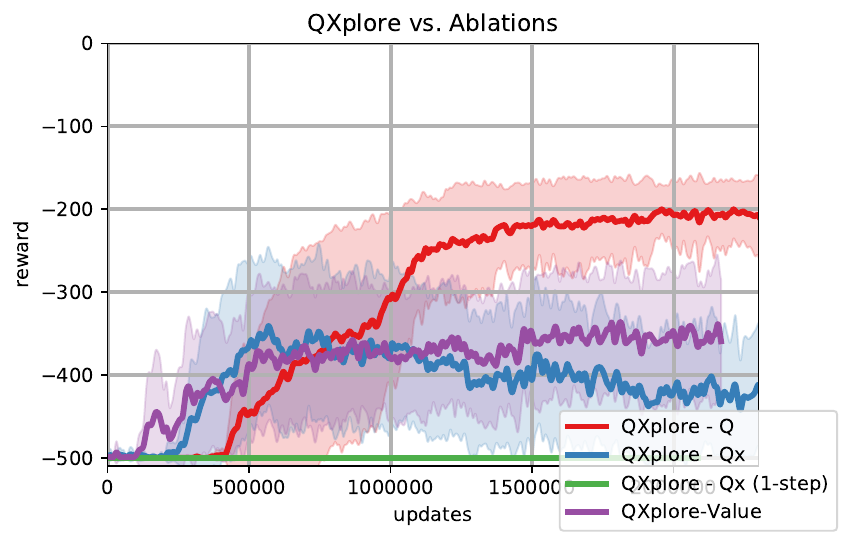}
    
% \caption{Plot showing the performance of $Q_x$ for QXplore with $\gamma_Q = 0.99$ (QXplore) and $\gamma_Q = 0$ (QXplore-near). In QXplore-near, $Q$ is trained with $\gamma$ of 0, and only predicts the reward of the current state-action pair. While QXplore-near is capable of finding reward through the state novelty fallback described in section \ref{subsec:0_predict}, it converges much slower.}
\caption{Plot showing the performance of two ablations, 1-Step Reward Prediction (QXplore-1-step) and Single-Policy QXplore (QXplore-value), compared to the original QXplore method. In the 1-Step ablation, $Q_x$ is trained to predict a combination of extrinsic reward and reward prediction error, and fails to make progress. In the Single-Policy ablation, the policy converges faster, but to a worse policy than vanilla QXplore due to the need to balance TD-error and extrinsic reward maximization.}
\label{fig:ablations}
\end{center}
 \vskip -0.1in
\end{figure}

Next, we tested a variant of QXplore using only a single sample policy and treating TD-error as a reward bonus, more in line with traditional exploration bonus methods. We trained a value function $V_{\theta}(s)$ trained via bootstrap and computed $r_x$ as $r_{x,\theta}(s_t,a_t,s_{t+1}) = |V_{\theta}(s_t) - (r_{\text{E}}(s_t,a_t) + {\gamma}V'_{\theta'}(s_{t+1}))|$. This variant uses only a single sample policy, $Q_x$, which is trained via bootstrapped off-policy Q-learning using one-step reward targets $r_1 = (r_x(s_t,a_t,s_{t+1}) + {\alpha}r_{\text{E}}(s_t,a_t)$
to maximize a combination of intrinsic and extrinsic rewards, controlled by the hyperparameter $\alpha$. We used $\alpha=0.1$, which we found to work well for \texttt{SparseHalfCheetah} in tuning experiments. We used a value function $V_{\theta}(s)$ rather than a Q-function for this ablation to avoid the wildly optimistic max action selection fully off-policy Q-functions have been reported to suffer from \citep{fujimoto2018off}. We label this experiment as ``QXplore-value'' in Figure \ref{fig:ablations}. This variant performs comparably to the $Q_x$ function of normal QXplore, but performance does not decrease late in training thanks to the extrinsic reward signal. However, overall performance is still well below that of normal QXplore's exploitation policy, which does not have to satisfy two conflicting training objectives.

\begin{figure}[ht]
%\vskip 0.2in
\begin{center}
\centering
\includegraphics[width=0.45\textwidth]{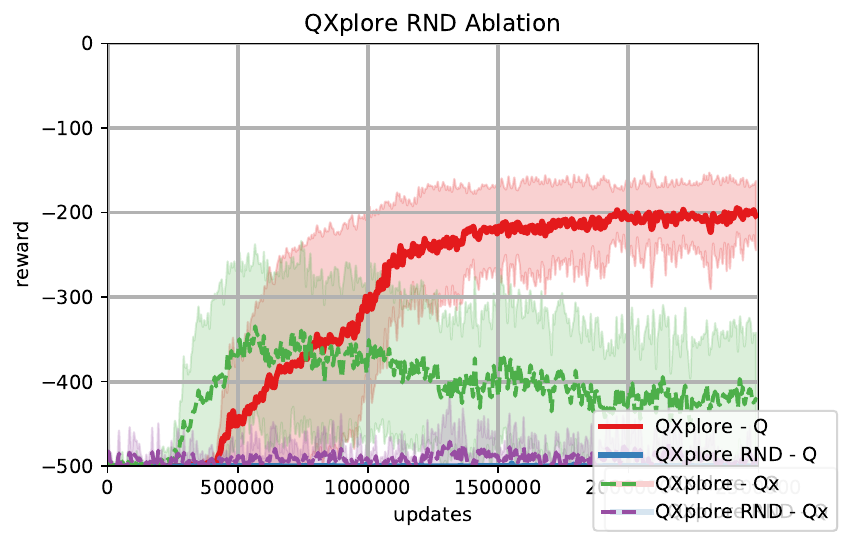}
\includegraphics[width=0.45\textwidth]{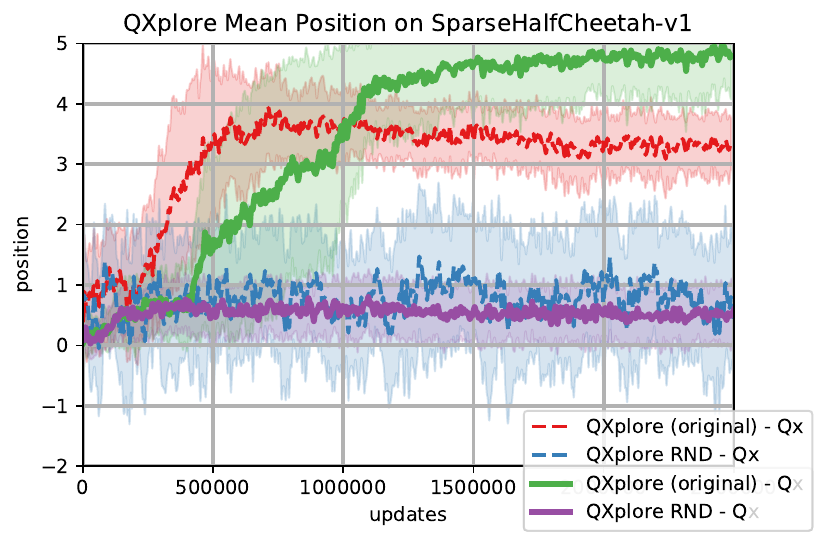}
\caption{Plots showing the performance of QXplore where the objective of $Q_x$ is replaced by the RND exploration objective, as well as the mean position of the cheetah during an episode throughout training. While $Q_x$ does sample reward, it does so too infrequently to guide $Q$ to learn the task. While the $Q_x$ function of QXplore-RND does reach states far from the origin, it does not display directional preference, whereas original QXplore's $Q_x$ function converges to sample states around the reward threshold at 5 units.}
\label{fig:qx_rnd}
\end{center}
 \vskip -0.1in
\end{figure}

Third, we tested a variant of QXplore where the TD-error maximization objective of $Q_x$ was replaced by the RND random network prediction error maximization objective. We call this ablation ``QXplore-RND'' and results are shown in Figure \ref{fig:qx_rnd} for both $Q$ and $Q_x$ policies. We observe that neither function converges to achieve reward. While we see that $Q_x$ does sample reward, $Q$ samples reward only during two episodes of training, and $Q_x$ does not converge to achieve high expected rewards itself. Looking at the mean position of the cheetah during an episode over training, we observe that for QXplore-RND $Q_x$ samples states relatively far from the origin compared to $Q$, based on the wider standard deviation, but does not display a directional preference (besides the inbuilt tendency to move forward more readily than backward that the cheetah has built in), since states found in both directions are equally novel. Comparatively, the $Q_x$ function of normal QXplore displays a strong forward preference once reward is found, and converges on sampling states close to the 5-unit reward threshold (this results in a mean position less than 5 due to time spent traveling from the origin), while the corresponding $Q$ function prefers to move well past the reward theshold (a mean position above 5) to reliably achieve reward.

\begin{figure}[ht]
%\vskip 0.2in
\begin{center}
\centering
\includegraphics[width=0.45\textwidth]{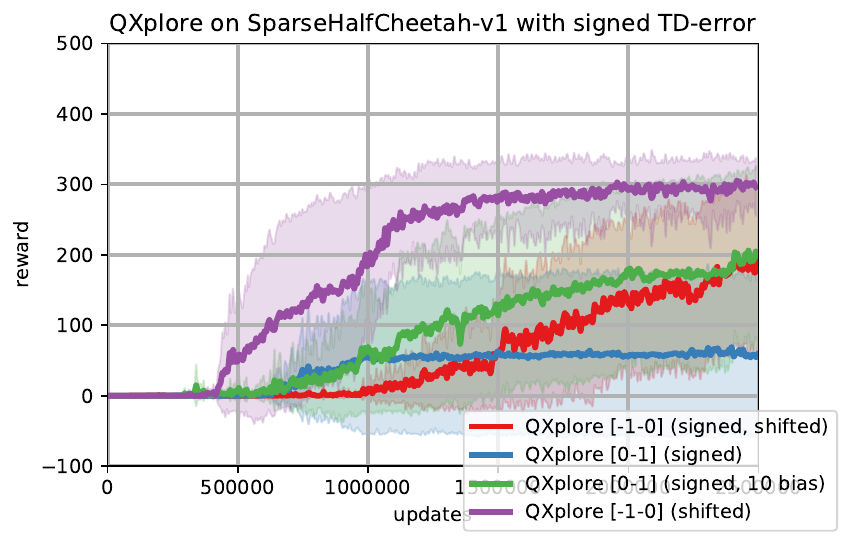}
\caption{The performance of QXplore's $Q$ function with $Q_x$ maximizing signed versus unsigned TD-error on two different reward variants of \texttt{SparseHalfCheetah}. While $Q$ is able to learn the task for all variants, performance is reduced with the signed objective. Performance on the \texttt{SparseHalfCheetah} variant with -1 to 0 reward function is shown shifted to match the axes of the 0 to 1 variant for comparison.}
\label{fig:signed_td}
\end{center}
 \vskip -0.1in
\end{figure}

Finally, we tested maximization of signed TD-error by $Q_x$ rather than unsigned. This objective tracks closer to dopamine-seeking in animals, where increases in dopamine (corresponding to an unexpectedly positive outcome) are sought out while decreases in dopamine (from unexpectedly negative outcomes) are avoided. To emulate this, we negate the signed TD error such that negative TD-error (the predicted Q-value was less than the target value) is maximized, while positive TD-error is minimized. $Q_x$ is otherwise trained as normal. The results are shown for both variants of the \texttt{SparseHalfCheetah} reward function (-1 to 0 and 0 to 1) in Figure \ref{fig:signed_td}, with and without setting the initial output bias of $Q$ to 10 in the 0 to 1 case. We observe that while QXplore does train with signed TD-error, performance is reduced. While this result bares further investigation, we hypothesize this is because prior to finding reward the sign of the TD-error is not correlated with the novelty of a state, thus the state novelty exploration phase is less efficient.

\section{Parameter Sweeps}
\label{appendix:param_sweeps}
We performed two sets of parameter sweeps for QXplore: varying the learning rates of $Q$ and $Q_x$, and varying the ratios of data sampled by each Q-function's policy used in training batches for each method. For learning rate, we tested combinations (QLR, QxLR) (0.01, 0.01), (0.01, 0.001), (0.001, 0.01), (0.001, 0.001), (0.001, 0.0001), (0.0001, 0.001), (0.0001, 0.0001). 

For batch data ratios, we tested combinations (specified as self-fraction for $Q$, then self-fraction for $Q_x$) of (0, 1), (0.25, 0.75), (0.5, 0.5), (0.75, 0.25).

Results for these sweeps can be seen in Figures \ref{fig:sweep_lr} and \ref{fig:sweep_rat}. QXplore is sensitive to learning rate, but relatively robust to the training data mix, to the point of $Q$ training strictly off-policy with only modest performance loss.

\begin{figure}[ht]
%\vskip 0.2in
\begin{center}

%\vskip 0.2in
    \begin{subfigure}[b]{0.45\textwidth}
        \centering
        \includegraphics[width=\textwidth]{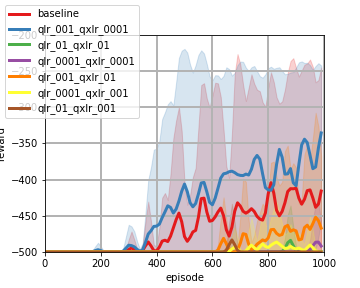}
        \caption{\label{fig:figg} SparseHalfCheetah}
    \end{subfigure}
        \begin{subfigure}[b]{0.45\textwidth}
        \centering
        \includegraphics[width=\textwidth]{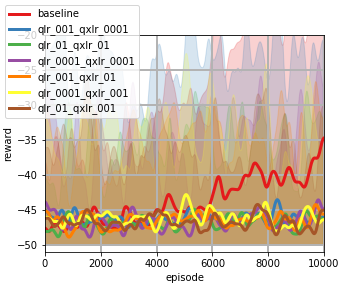}
        \caption{\label{fig:figh} FetchPush-v1}
    \end{subfigure}
    
\caption{Learning rate sweeps for $Q$ and $Q_x$}
\label{fig:sweep_lr}
\end{center}
% \vskip -0.4in
\end{figure}

\begin{figure}[ht]
%\vskip 0.2in
\begin{center}

%\vskip 0.2in
    \begin{subfigure}[b]{0.45\textwidth}
        \centering
        \includegraphics[width=\textwidth]{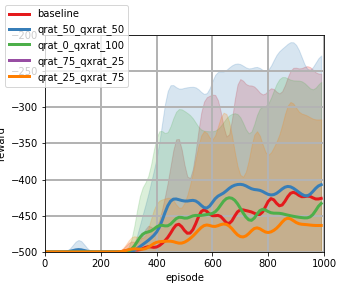}
        \caption{\label{fig:figi} SparseHalfCheetah}
    \end{subfigure}
        \begin{subfigure}[b]{0.45\textwidth}
        \centering
        \includegraphics[width=\textwidth]{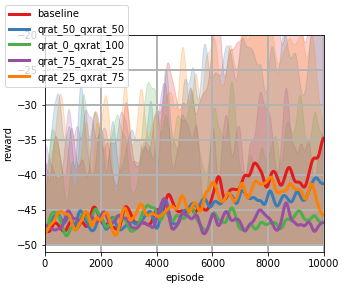}
        \caption{\label{fig:figj} FetchPush-v1}
    \end{subfigure}
    
\caption{Sample ratio sweeps for $Q$ and $Q_x$}
\label{fig:sweep_rat}
\end{center}
% \vskip -0.4in
\end{figure}

\subsection{RND Parameter Sweeps}
\label{appendix_subsec:rnd_sweeps}

As we have adapted RND to operate with vector observations and continuous actions, we performed several hyperparameter sweeps to ensure a fair comparison. We report in Figure \ref{fig:rnd_sweeps} the results of varying both predictor network learning rate ``lr'' and extrinsic reward weight ``rw'' independently on the \texttt{SparseHalfCheetah} task. The baseline values for these parameters used elsewhere are 0.001 and 2 respectively. We observe that RND is fairly sensitive to reward weight, but a value of 1 or two performs well, while a learning rate of 0.001 appears to learn faster early in training without loss of final performance.

\begin{figure}[ht]
%\vskip 0.2in
\begin{center}
        \centering
        \includegraphics[width=\textwidth/2]{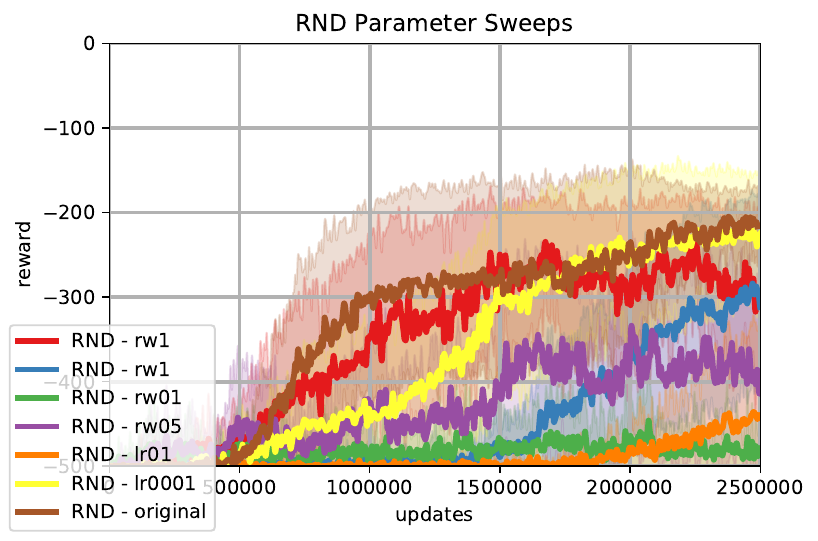}
\caption{Parameter sweeps for RND. A reward weight of either 1 or 2 works best, with a learning rate of 0.0001 a close second.}
\label{fig:rnd_sweeps}
\end{center}
% \vskip -0.4in
\end{figure}

\section{Reward Shifting versus $\beta_Q$}
\label{appendix:01_reward}
For most of our experiments with the \texttt{SparseHalfCheetah} environment, we used a reward function that is -1 for non-goal states and 0 for goal states to have consistent reward shaping with the \texttt{Fetch} tasks in the OpenAI Gym. However, as the original \texttt{SparseHalfCheetah} proposed by \cite{houthooft2016vime} used a reward function that is 0 for non-goal states and 1 for goal states, we present results for QXplore and our implementation of RND on the original reward function as well in Figure \ref{fig:01_reward}. Because we initialized the output distribution $Q$ to be close to 0 initially, QXplore performed worse on this reward function due to the much smaller magnitude of TD-errors during the initial reward-free exploration phase slowing down exploration. However, adjusting the hyperparameter $\beta_Q$, the initial bias of the output neuron of $Q$, allows us to obtain identical performance to the -1 to 0 reward function. QXplore's state novelty search efficiency is sensitive to this initial TD-error magnitude, which varies depending on the reward function, but in a coarse parameter sweep of initial biases of -10, 0, 1, 10, and 100 we found a good setting for the parameter which performed comparably to the -1 to 0 reward function. This dependency is similar in concept to the reward weighting used by many reward bonus methods to trade off between exploration and exploitation, the setting of which may also depend on the reward landscape.

\begin{figure}[ht]
%\vskip 0.2in
\begin{center}
\centering
\includegraphics[width=0.45\textwidth]{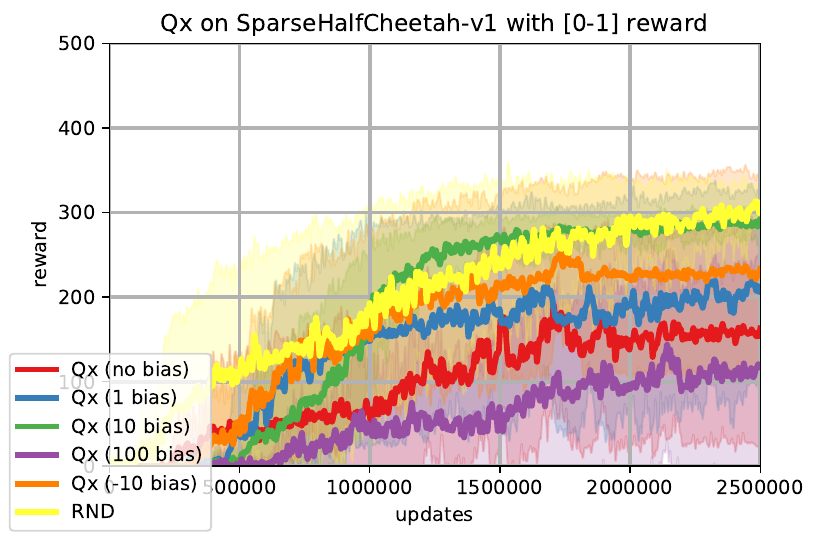}
\caption{QXplore performance on \texttt{SparseHalfCheetah} with the 0 to 1 reward function. Adjusting $\beta_Q$ recovers full performance compared to the -1 to 0 reward function (shown here shifted by 500 reward for comparison). We tested several different values for $\beta_Q$ and found that a value of 10 worked best for \texttt{SparseHalfCheetah}.}
\label{fig:01_reward}
\end{center}
 \vskip -0.1in
\end{figure}

\section{The `Noisy TV' Problem}
\label{appendix:noisy_tv}
The `Noisy TV' problem is a classic issue with some state-novelty exploration methods in which states with unpredictable observations serve as maxima in the novelty reward space. QXplore's TD-error objective is not fundamentally vulnerable to the problem, but to demonstrate that our function approximation early in training is also no subject to it, we trained QXplore on a variant of the \texttt{SparseHalfCheetah} task where we add a random normally-distributed value to the observation vector of the agent. The variance of this noise value increases proportionately to the movement of the cheetah in the negative direction (away from the reward threshold). An agent vulnerable to the noisy tv problem will be enticed to explore in the negative direction rather than forward, as this maximizes the novelty/unpredictability of the observations. 

We show the results of training QXplore on this environment in Figure \ref{fig:randobs} for both $Q$ and $Q_x$, as well as the mean position of the cheetah along the movement dimension during $Q_x$'s training rollouts. As expected, the performance of neither $Q$ nor $Q_x$ is meaningfully altered relative to the baseline, and $Q_x$ is not biased to explore backwards to a greater degree than it typically does early in training.

\section{Weight Initialization}
\label{appendix:initialization}
As we use neural net function approximation error as a state novelty baseline for early exploration, the behavior of $Q_x$ may be sensitive to weight initialization. To test this, in addition to the Pytorch default initialization method ``Kaiming-Uniform,'' \citep{he2015delving} which we used for all runs outside this section, we also tested initializing both $Q$ and $Q_x$ with ``Kaiming-Normal'' and ``Xavier-Uniform,'' \citep{glorot2010understanding} two other initialization methods that result in higher variance between initial outputs of the networks, which translates into reduced training performance. We further tested two naive distributions that produced very high variance in outputs, ``Normal,'' sampling weight values from $\mathbf{N}(0,1)$ and ``Uniform,'' sampling values from $\mathbf{U}(-1, 1)$. These configurations were not expected to perform as well as ``Kaiming-Uniform'', but do test the ability of $Q_x$ to explore given a poor initialization. In all cases other than ``Kaiming-Uniform'' we set the bias of each neuron to 0. The results of QXplore with each initialization scheme on \texttt{SparseHalfCheetah} are shown in Figure \ref{fig:weight_init}. 
%We also include RND with the Q-function (but not predictor or random network) initialized using two of the suboptimal initialization schemes as a baseline for initialization sensitivity.

``Kaiming-Normal'' and ``Xavier-Uniform'' both showed moderate decrease in overall performance, though both $Q$ and $Q_x$ were able to converge on reward. ``Normal'' and ``Uniform'' however both more-or-less prevented $Q$ from converging on reward. Their effect on the ability of $Q_x$ to find reward however is much more mild- only ``Normal'' and to a lesser extent ``Uniform'' caused significant issues with discovering and converging on reward. This suggests that $Q_x$ is not particularly dependent on careful weight initialization to explore with function approximation error.

\begin{figure}[ht]
%\vskip 0.2in
\begin{center}

%\vskip 0.2in
\begin{subfigure}[b]{0.45\textwidth}
    \centering
    \includegraphics[width=\textwidth]{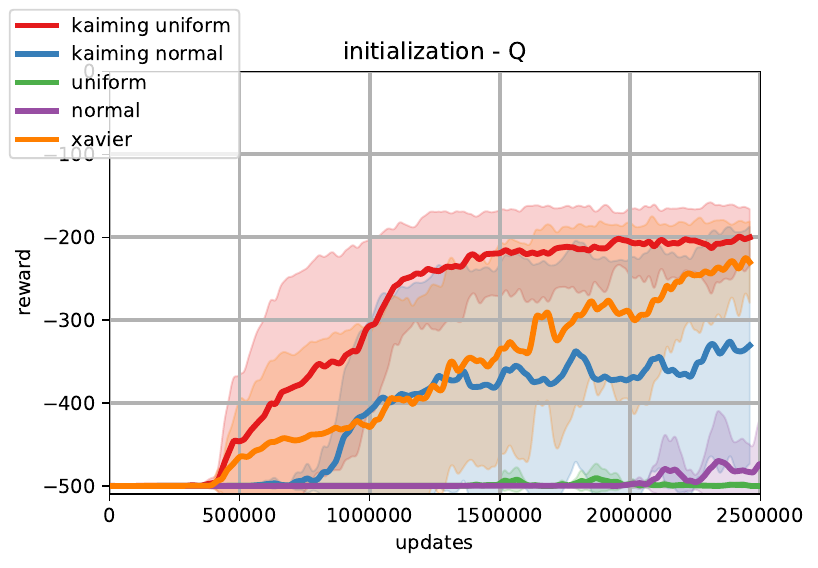}

    \caption{\label{fig:figk} Initialization of $Q$}
\end{subfigure}
    \begin{subfigure}[b]{0.45\textwidth}
    \centering
    \includegraphics[width=\textwidth]{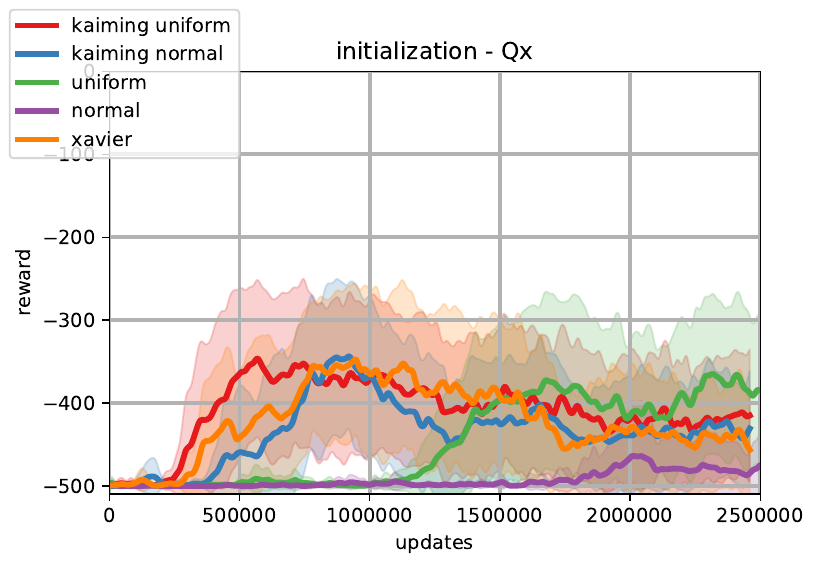}
    \caption{\label{fig:figl} Initialization of $Q_x$}
\end{subfigure}

\caption{Several alternate initialization schemes for $Q$ and $Q_x$. While $Q$ is adversely impacted, $Q_x$ is relatively robust even to very poor initializations such as ``Normal'' and ``Uniform.''}
\label{fig:weight_init}
\end{center}
 \vskip -0.1in
\end{figure}
\begin{figure}[ht]
%\vskip 0.2in
\begin{center}

%\vskip 0.2in
\begin{subfigure}[b]{0.45\textwidth}
    \centering
    \includegraphics[width=\textwidth]{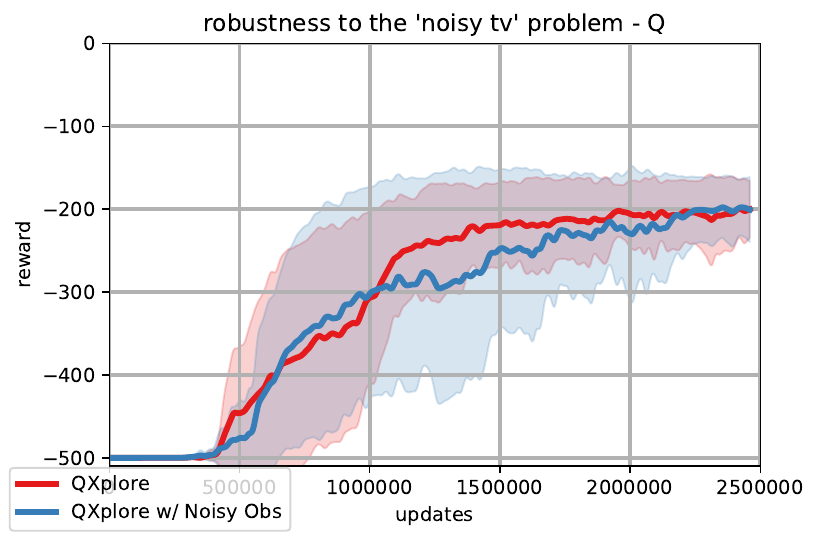}

    \caption{\label{fig:figm} Noisy observation effects on $Q$}
\end{subfigure}
\begin{subfigure}[b]{0.45\textwidth}
    \centering
    \includegraphics[width=\textwidth]{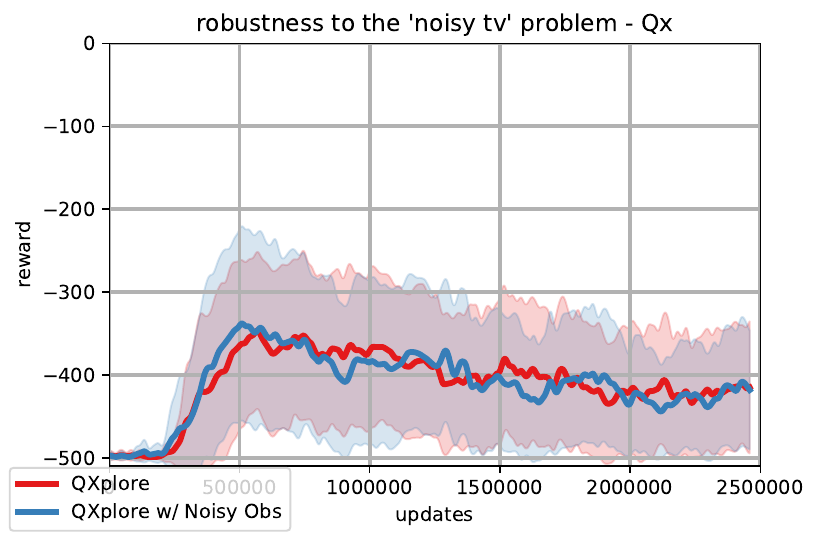}
    \caption{\label{fig:fign} Noisy observation effects on $Q_x$}
\end{subfigure}
\\
\begin{subfigure}[b]{0.45\textwidth}
    \centering
    \includegraphics[width=\textwidth]{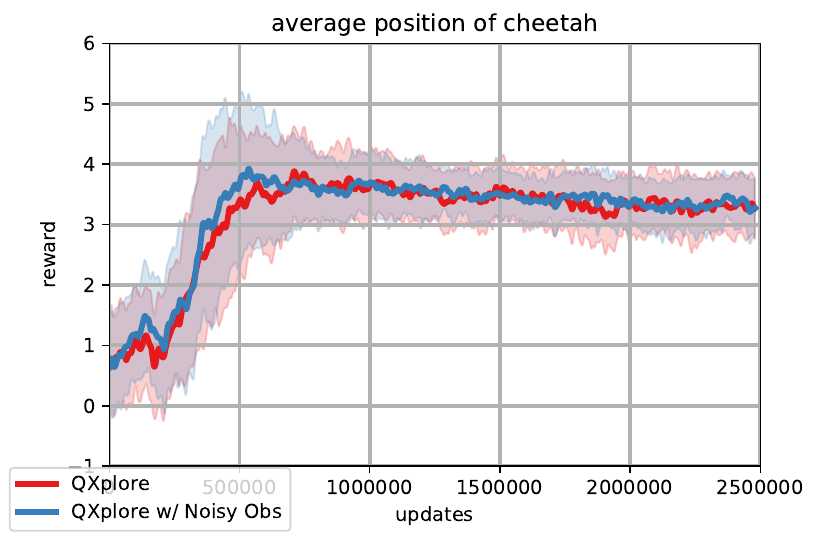}
    \caption{\label{fig:figo} Noisy observation effects on absolute position}
\end{subfigure}

\caption{QXplore trained on a `noisy tv' variant of \texttt{SparseHalfCheetah} where one element of the observation vector is normally distributed random value whose variance increases if the cheetah moves in the negative direction. The performance of QXplore is not impacted in any way by this noise, and it trains as normal.}
\label{fig:randobs}
\end{center}
 \vskip -0.1in
\end{figure}
